# Supplementary material for: Taming Consistency Distillation for Accelerated Human Image Animation
Source: arXiv:2504.11143 source file (2025-04-15)
Supplement: Supplementary file 1 [file X_suppl.tex]

\clearpage
\appendix

\twocolumn[
% \maketitlesupplementary
{
% \maketitle
% \twocolumn[
        \centering
        \Large
        \textbf{\thetitle}\\
        \vspace{0.3em}Supplementary Material \\
        \vspace{1.5em}
        % {
        % \small
        % \iftoggle{cvprrebuttal}{}{
        %       Anonymous \confName~submission\\
        %       \vspace*{1pt}\\
        %       Paper ID \paperID \\
        %     }
        %     }
        % \vspace{1.5em}
       % ] %< twocolumn
% \maketitlesupplementary
    \centering
    \vspace{5pt}
    \includegraphics[width=1.00\textwidth]{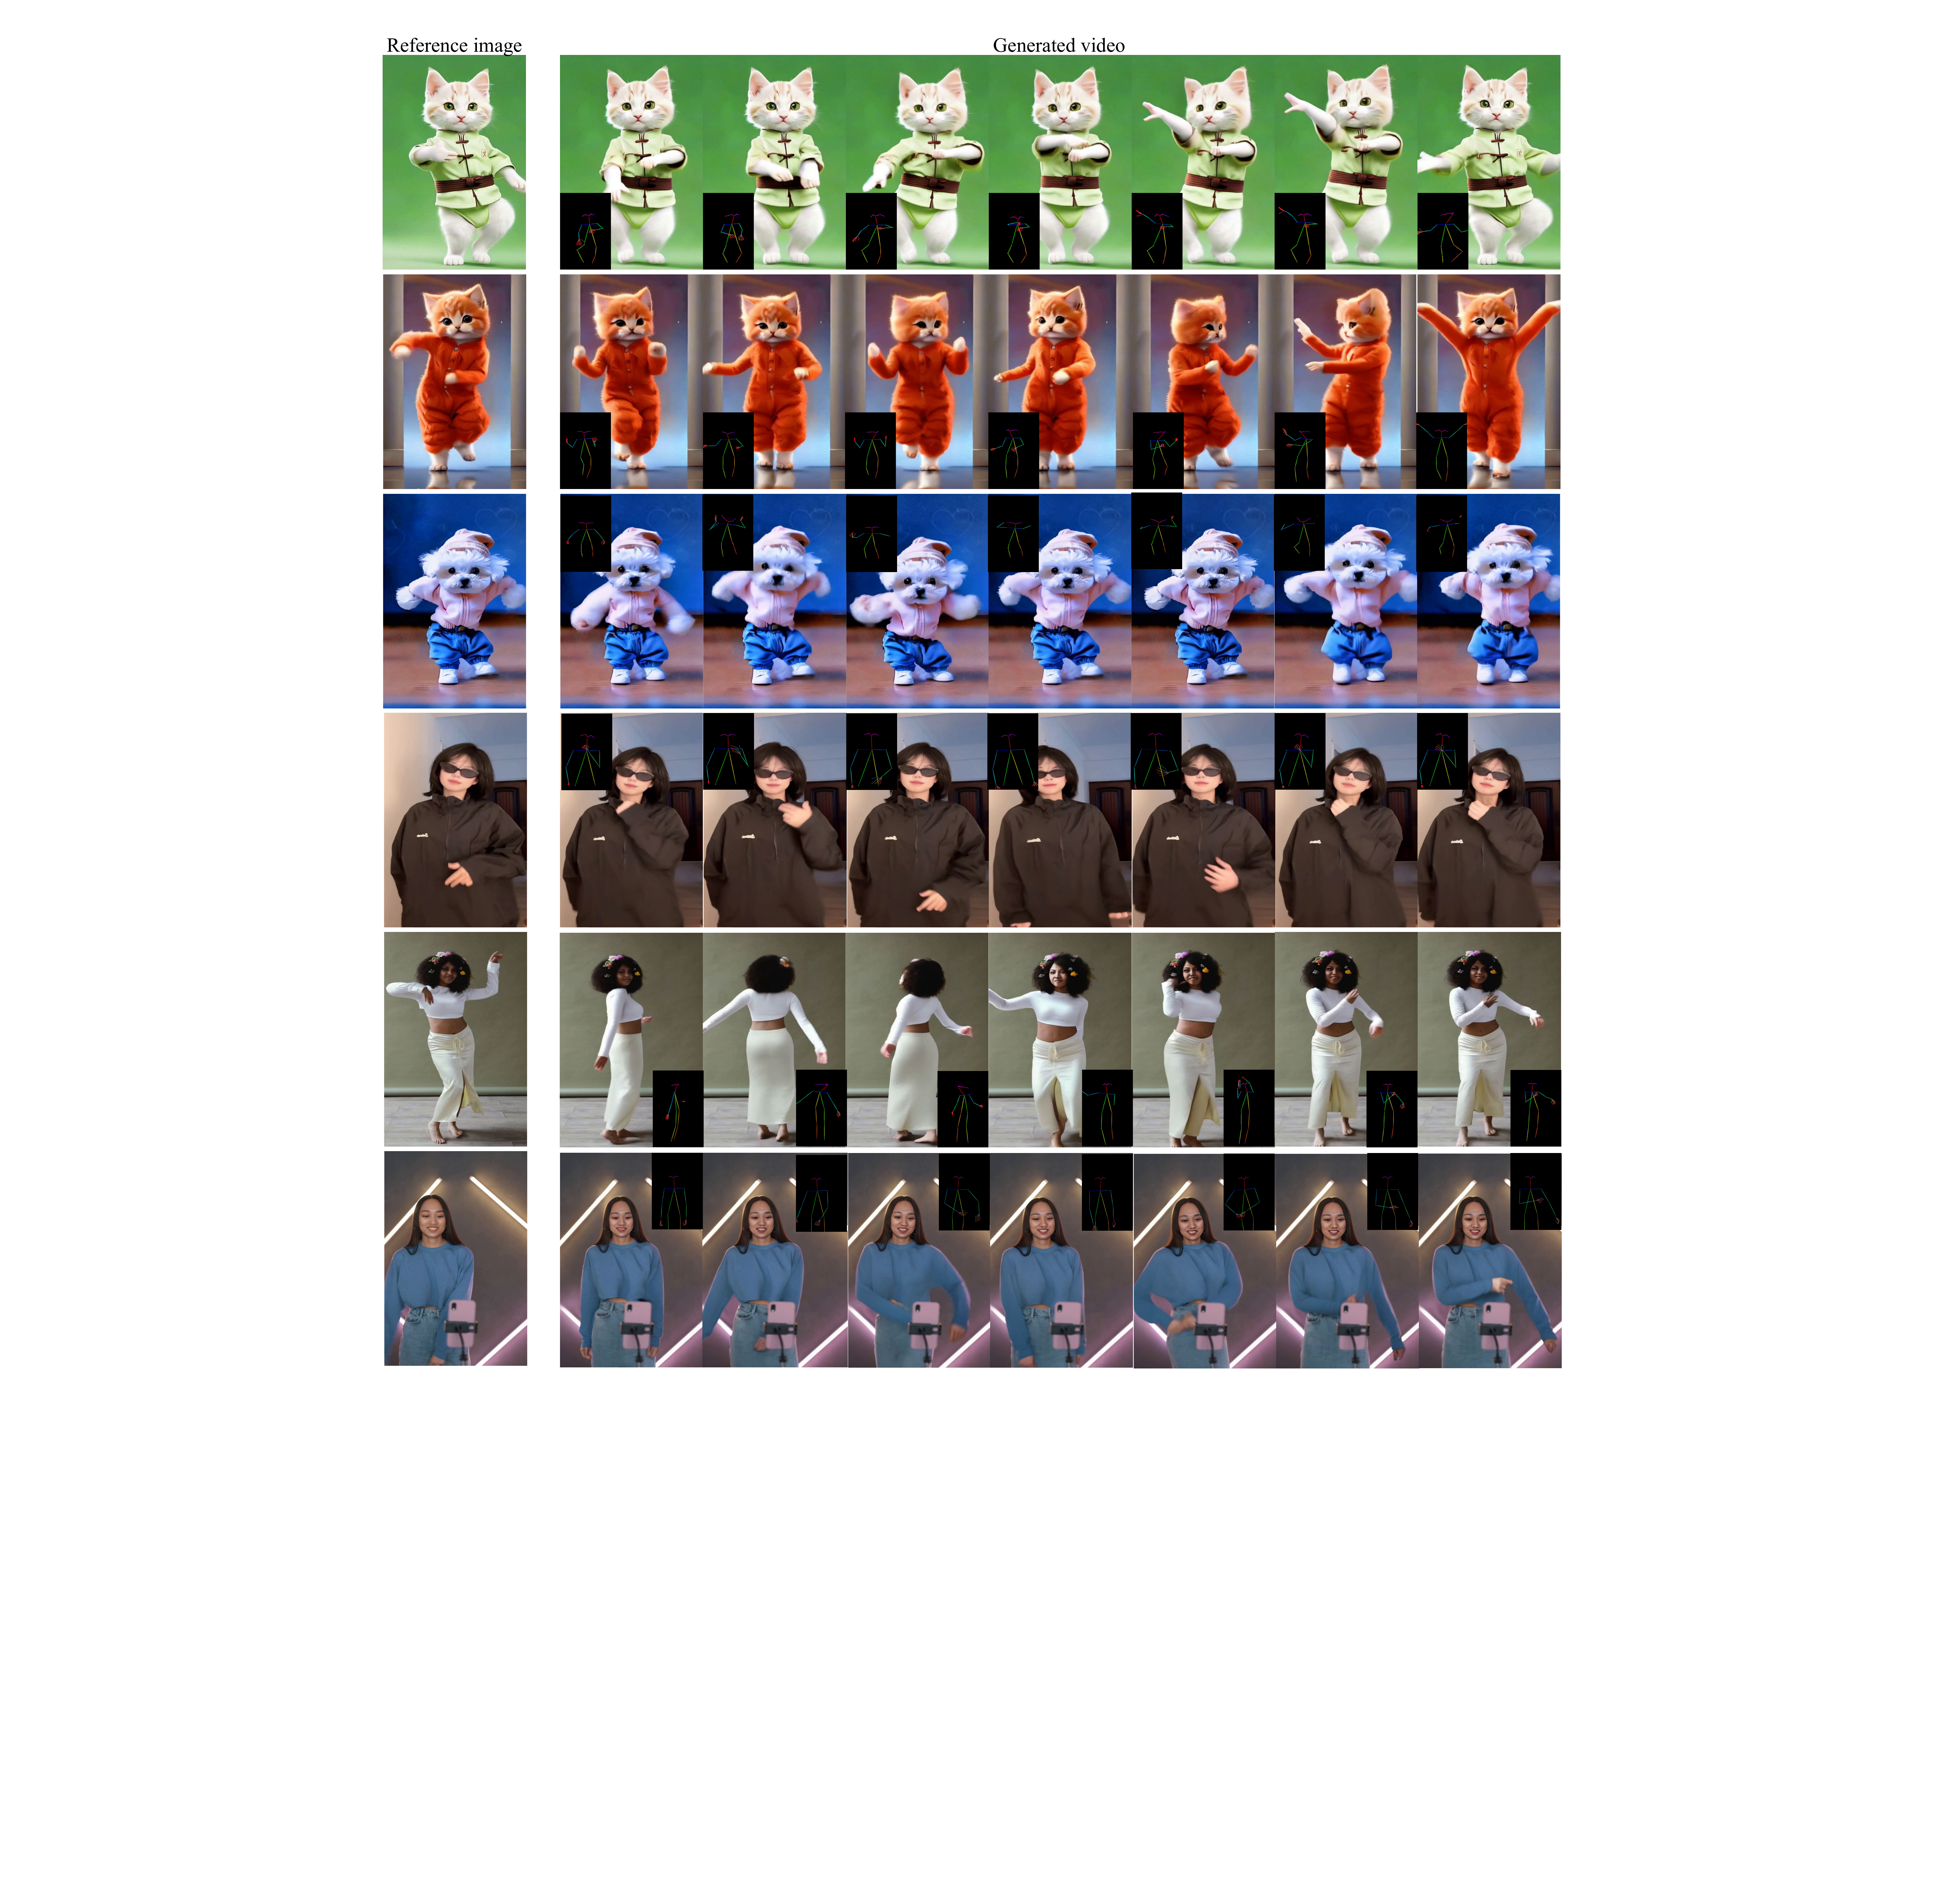}
    \vspace{-28pt}
    \captionof{figure}{
        More qualitative visualization results generated by the proposed \method.
        %
        % Since only language-free videos are required, High-definition videos can be easily generated.
        % High-definition videos can be 
        %
    }
    \label{first_figure_supp}
    \vspace{18pt}
    }
]

% Due to page limitations, we move some parts
Due to page limitations of the main paper, we add more experimental details and results in this appendix.
%
% In addition, 
% Besides,
% limitations and future work will also be discussed.
%

\begin{table}[t]
    % \vspace{-1.1em}
    \small
    % \tablestyle{4pt}{0.95}
    % \vspace{-5pt}
    \centering
    \setlength{\tabcolsep}{13pt}{
   % \begin{tabular}{@{}lc@{}}
   % \resizebox{\textwidth}{20mm}{
   % \scalebox{0.98}{
      \begin{tabular}{l|c}
    \shline
      \hspace{-4mm}  Comparison settings       &  Human preference \\
        \shline
      \hspace{-4mm}  \method vs. VideoLCM~\cite{wang2023videolcm}   &  \textbf{82.0\%} vs. 18.0\%   \\
      \hspace{-4mm}  \method vs. PeRFlow~\cite{yan2024perflow}  &   \textbf{68.0\%} vs. 32.0\%      \\
     \hspace{-4mm}   \method vs. Multistep CM~\cite{heek2024multistep}  & \textbf{61.0\%} vs. 39.0\%     \\
       \shline
    \end{tabular}
    }
    % \vspace{-10pt}
    \vspace{-3mm}
    \caption{
        {
        Human preference on different acceleration algorithms. The experiment are carried out under 4-step denoising inference. 
    }}
    % }
     \label{tab:human_perference}
     \vspace{-1mm}
% \end{wraptable}
\end{table}

% \vspace{-4mm}
%
\begin{table}[t]
\centering
\small
% \normalsize
% \large
% \tablestyle{5pt}{1.1}
\setlength{
    \tabcolsep}{
    4.8mm}{
\begin{tabular}
{l|c}
\hline			
\hspace{-0.8mm}  \multirow{1}{*}{Method}  & Identity Similarity \\
\shline
VideoLCM & 0.189  \\
+ CLIP face feature & 0.227 \\
+ VAE face feature \textbf{(Ours)} & \textbf{0.342} \\
% \multicolumn{1}{c|}{{\emph{w/o} temporal coherence loss}} & \multicolumn{1}{c}{{TF-T2V}}    \\
% \hspace{-1mm} ID Similarity & 0.181 & 0.279 & \textbf{0.419}  \\ 
\hline

\end{tabular}
}
\vspace{-2mm}
\caption{
% Quantitative 
% Cosine similarity between real and predicted faces on TikTok.
%
Quantitative results of ArcFace similarity on TikTok.
}
\label{tab:face}
\vspace{-2mm}
\end{table}

% \vspace{-4mm}
%
\begin{table*}[t]
\centering
\small
% \normalsize
% \large
% \tablestyle{5pt}{1.1}
\setlength{
    \tabcolsep}{
    5.0mm}{
\begin{tabular}
{l|c|cccc}
\hline			
\hspace{-0.8mm}  \multirow{1}{*}{Method}  & Steps & L1 $\downarrow$  &   SSIM $\uparrow$   & LPIPS $\downarrow$ & FVD $\downarrow$ \\
% \multicolumn{1}{c|}{{\emph{w/o} temporal coherence loss}} & \multicolumn{1}{c}{{TF-T2V}}    \\

\shline

\hspace{-1mm} MagicAnimate (teacher)~\cite{magicanimate} & 25  & 3.13E-04 & 0.714 & 0.239 & 179.07 \\ 
\hline
\hspace{-1mm} VideoLCM~\cite{wang2023videolcm} & 4  & 3.21E-04 & 0.594 & 0.264 & 265.99 \\ 
\hspace{-1mm} \textbf{\method} & \textbf{4}  &  \textbf{2.88E-04} & \textbf{0.744} & \textbf{0.231} &  \textbf{177.32} \\

\hline

\end{tabular}
}
\vspace{-2mm}
\caption{
% Quantitative 
Comparisons based on the MagicAnimate framework. We leverage MagicAnimate as the teacher model to distill our \method.
}
\label{tab:magic}
\vspace{1mm}
\end{table*}
% \end{figure*}

% \vspace{-4mm}
%
\begin{table*}[t]
\centering
\small
% \normalsize
% \large
% \tablestyle{5pt}{1.1}
\setlength{
    \tabcolsep}{
    2.7mm}{
\begin{tabular}
{l|ccccc}
\hline			
\hspace{-0.8mm}  \multirow{1}{*}{Method}  & MagicAnimate~\cite{magicanimate} & Anymate Anyone~\cite{Animateanyone} & Champ~\cite{champ} &   UniAnimate~\cite{wang2024unianimate}   & \textbf{\method} \\
% \multicolumn{1}{c|}{{\emph{w/o} temporal coherence loss}} & \multicolumn{1}{c}{{TF-T2V}}    \\

\shline

\hspace{-1mm} Steps & 25 & 20 & 20 & 50   & \textbf{4}    \\ 
\hspace{-1mm} Latency & 32.1s  & 36.8s & 28.5s & 46.7s  &\textbf{4.1s}  \\

\hline

\end{tabular}
}
\vspace{-2mm}
\caption{
% Quantitative 
Latency comparison with baselines on one A800 GPU.
}
\label{tab:speed}
\vspace{-2mm}
\end{table*}

\section{Additional experimental details}

In our experiments, 
UniAnimate~\cite{wang2024unianimate} is leveraged as the teacher diffusion model for knowledge distillation.
Our consistency distillation is conducted on a latent space, and
an off-the-shelf pre-trained variational
autoencoder (VAE) model~\cite{guo2023animatediff} from Stable Diffusion 2.1~\cite{stablediffusion} is used to obtain the latent features.
The downsample factor of the VAE encoder is 8.
The model structure of  \method is basically the same as that of UniAnimate except that we introduce an additional auxiliary head and inject coefficient information of the classifier-free guidance into the model by adding it to the time embedding like LCM~\cite{luo2023latent}.
% The model structure of \method is basically the same as that of UniAnimate and C to facilitate fair comparison.
%
To further demonstrate the generalizability of our approach, MagicAnimate is also leveraged as a teacher model to train our approach.
% In the experiment,
% the network structure of \method is basically consistent with the open source ModelScopeT2V and VideoComposer to facilitate fair comparison.
%
% Note that \method is a plug-and-play framework that can also be applied to other text-to-video generation and controllable video synthesis methods.
%
%
% \method support different resolutions as input
% As for human evaluation, we randomly generated 100 videos and asked users to 
% [Details about user study]
%
% For human evaluation, we randomly generate 100 videos and ask users to rate and evaluate them. The highest score for each evaluation content is 100\%, the lowest score is 0\%, and the final statistical average is reported.

\section{More experimental results}

\noindent\textbf{More qualitative results.}
As displayed in \cref{first_figure_supp}, we show the additional qualitative results of the proposed \method on the human image animation task with four inference steps.
From the results, we can observe that
\method achieves visually appealing and temporally coherent results.
% than the baseline VideoComposer.
%
%
% In particular, we notice that our method is also well adapted to possible interference factors such as wearing glasses.
%
% In addition, we can find that our model also generalizes well for some animals, such as cats and dogs.
% \hangjie{
Notably, we observe that our method effectively adapts to cases with potential interference factors, such as subjects wearing glasses.
Furthermore, our model demonstrates strong generalization to animals, including cats and dogs.
% }

\vspace{1mm}
\noindent\textbf{Human preference.}
To further evaluate the performance of the proposed \method compared to the previous acceleration methods~\cite{wang2023videolcm,yan2024perflow,heek2024multistep}, we randomly sample 50 reference images and feed them to these models to generate videos.
The generated results are evaluated by 4 different human raters.
The results of human preference are shown in ~\cref{tab:human_perference}.
From the results, We can clearly see that our method is superior to other acceleration algorithms.
Specifically, our \method achieves a human preference rate of 82.0\% compared to VideoLCM, indicating the effectiveness of the proposed components. 

% \section{Additional ablation study}

\vspace{1mm}
\noindent
\textbf{Quantitative evaluations of enhanced facial fidelity.}
To indicate the effectiveness of incorporating face condition, we compare the facial fidelity.
~\cref{tab:face} shows cosine similarity between real and predicted video faces, and our method helps to improve facial fidelity.
% Thanks for the suggestion. From the results in ~\cref{tab:face}, we find that our method helps to improve facial fidelity.

\vspace{1mm}
\noindent
\textbf{Train LCM model on more animation frameworks.}
{%
To further demonstrate the generalizability of our approach, we also use MagicAnimate as a teacher model to train our approach.
% Thanks for pointing out this.
% Thanks.
As shown in Tab.~\ref{tab:magic} and Fig.~\ref{fig:Magic}, 
we observe the superior performance of our DanceLCM over VideoLCM, matching or even exceeding the teacher method MagicAnimate, indicating the generalization of our method.
% we can find that our can 
% show the results based on MagicAnimate
}

\vspace{1mm}
\noindent
\textbf{Inference speed comparison 
 with prior works.}
\noindent
{%
% extra latency comparison
% Thanks. % for the suggestion.
As stated before, our method can accelerate existing human image animation methods.
We add latencies for generating 32-frame videos in Tab.~\ref{tab:speed}. From the results, we can find that our \method can significantly reduce the inference latency compared to other existing diffusion-based methods.
}

\begin{figure}[t]
    \centering
    \vspace{-2mm}\includegraphics[width=0.99\linewidth]{Picture_supp/rebuttal_2.pdf}
    \vspace{-2mm}
    \caption{Qualitative comparisons based on MagicAnimate.}
    \label{fig:Magic}
    \vspace{-1mm}
\end{figure}
