# Supplementary material for: Taming Consistency Distillation for Accelerated Human Image Animation
Source: arXiv:2504.11143 source file (2025-04-15)
Supplement: Supplementary file 2 [file X_suppl_arxiv.tex]

\clearpage

\twocolumn[
% \maketitlesupplementary
{
% \maketitle
% \twocolumn[
        \centering
        \Large
        \textbf{\thetitle}\\
        \vspace{0.3em}Supplementary Material \\
        \vspace{1.5em}
    \centering
    \vspace{5pt}
    \includegraphics[width=1.00\textwidth]{Picture_supp/Compare_mv_small.pdf}
    \vspace{-28pt}
    \captionof{figure}{
        \textbf{Qualitative comparison on compositional motion-to-video synthesis}. The videos are generated by taking textual descriptions
and motion vectors as conditions. Compared to VideoComposer, TF-T2V produces more realistic and appealing results.
        %
        % Since only language-free videos are required, High-definition videos can be easily generated.
        % High-definition videos can be 
        %
    }
    \label{first_figure_supp}
    \vspace{18pt}
    }
]

% \end{figure*}

% Due to page limitations, we move some parts
Due to the page limit of the main text, we add more details and experimental results in this appendix.
%
% In addition, 
Besides,
limitations and future work will also be discussed.

\begin{table}[t]
    % \vspace{-1.1em}
    \caption{
        {
        Ablation study on different training manners. 
    }}
     \label{tab:compare_with_train_manner}
     \vspace{-3mm}
    \tablestyle{4pt}{0.95}
    % \vspace{-5pt}
    \centering
    \setlength{\tabcolsep}{10pt}{
   % \begin{tabular}{@{}lc@{}}
   % \resizebox{\textwidth}{20mm}{
   % \scalebox{0.98}{
      \begin{tabular}{l|ccc}
    \shline
        Setting       &  FID ($\downarrow$) &   FVD  ($\downarrow$)  & CLIPSIM ($\uparrow$) \\
        \shline

        Separately   &  9.22 & 503 & 0.2905 \\
        \rowcolor{Gray}
        Jointly  &   \textbf{8.19}  & \textbf{441}  & \textbf{0.2991}  \\
        % \shline
       \shline
    \end{tabular}
    }
    % \vspace{-10pt}
    \vspace{-3mm}
% \end{wraptable}
\end{table}

\section{More experimental details}

In \cref{first_figure_supp}, we show the comparison on compositional motion-to-video synthesis.
\method achieves more appealing results than the baseline VideoComposer.
Following prior works, 
we use an off-the-shelf pre-trained variational
autoencoder (VAE) model from Stable Diffusion 2.1 to encode the latent features.
The VAE encoder has a downsample factor of 8.
% The model structure of A is basically the same as that of B and C to facilitate fair comparison.
%
In the experiment,
the network structure of \method is basically consistent with the open source ModelScopeT2V and VideoComposer to facilitate fair comparison.
Note that \method is a plug-and-play framework that can also be applied to other text-to-video generation and controllable video synthesis methods.
%
% To verify the high-definition generation capability of \method, we train 
% To verify that \method can be extended to high-definition video generation, we also use text-free videos to train a high-resolution text-to-video model, such as $896\times512$. For high-definition compositional video synthesis, we synthesize $1280\times640$ and $1280\times768$ videos to demonstrate the excellent application potential of our method.
%
% \method support different resolutions as input
% As for human evaluation, we randomly generated 100 videos and asked users to 
% [Details about user study]
For human evaluation, we randomly generate 100 videos and ask users to rate and evaluate them. The highest score for each evaluation content is 100\%, the lowest score is 0\%, and the final statistical average is reported.

\section{Additional ablation study}
